# Supplementary material for: Generalized Contact Formalism Analysis of the $^4$He$(e,e'pN)$ Reaction
Source: arXiv:2003.02318 source file (2020-04-11)
Supplement: Supplementary file 1 [file GCF_Supplementary_V2.pdf]

<u>Supplementary materials for:</u> "Generalized Contact Formalism Analysis of Exclusive Short-Range Correlations Measurements Using The $^4$He(e,e'pN) Reaction "

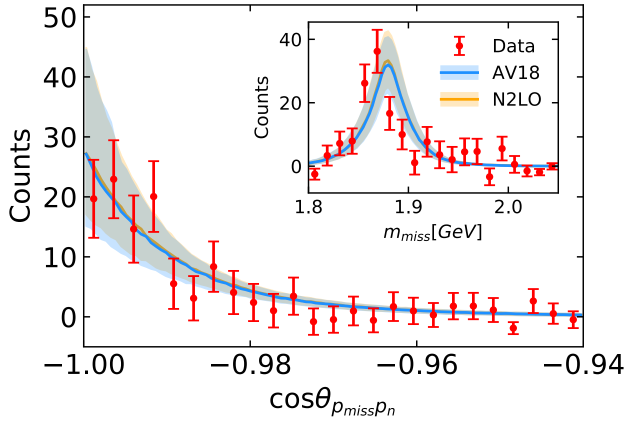


**Supplementary Materials Fig. 1:** Same as Fig. 1 in the main text for light-cone GCF calculation.

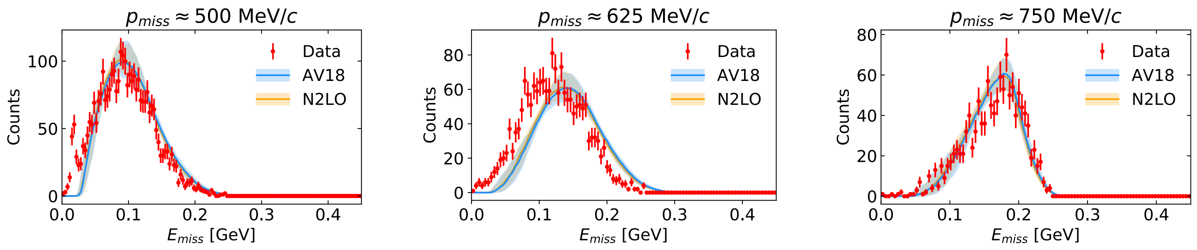


**Supplementary Materials Fig. 2:** Same as Fig. 2 in the main text for light-cone GCF calculation.

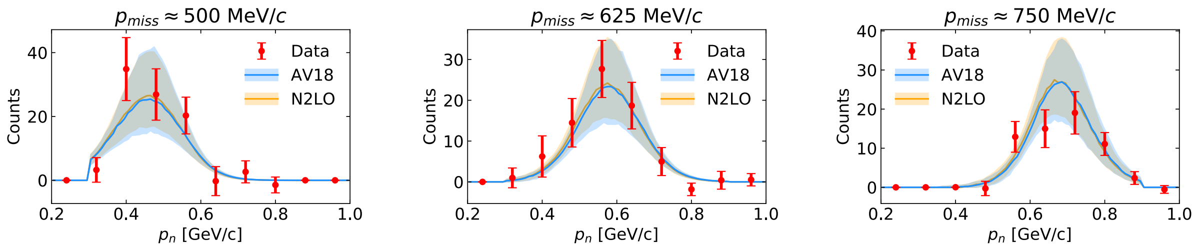


**Supplementary Materials Fig. 3:** Same as Fig. 3 in the main text for light-cone GCF calculation.

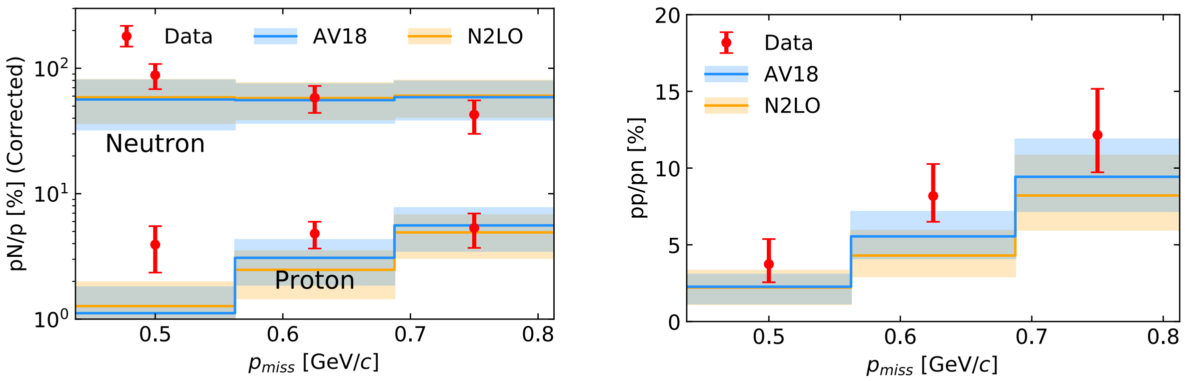


**Supplementary Materials Fig. 4:** Same as Fig. 4 in the main text for light-cone GCF calculation.

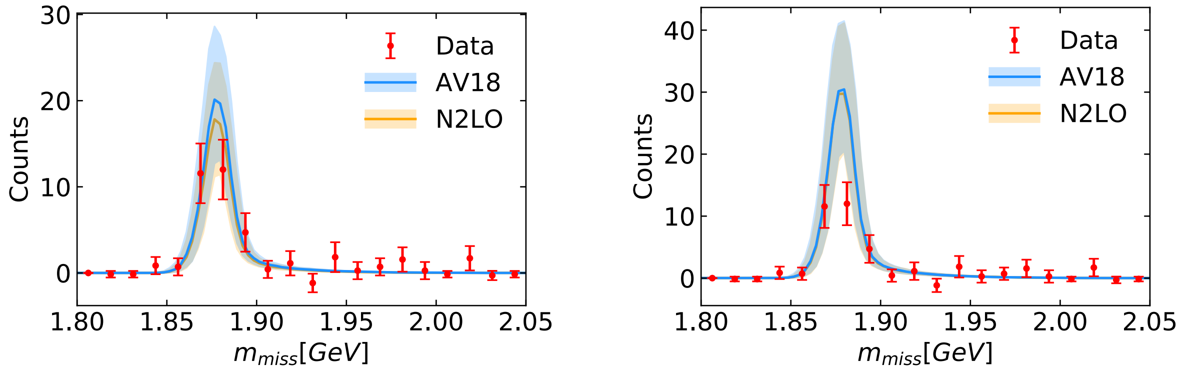


**Supplementary Materials Fig. 5:** $^4$He(e,e'pp) missing mass. Data are compared with both light-cone (left) and instant form (right) GCF calculations.

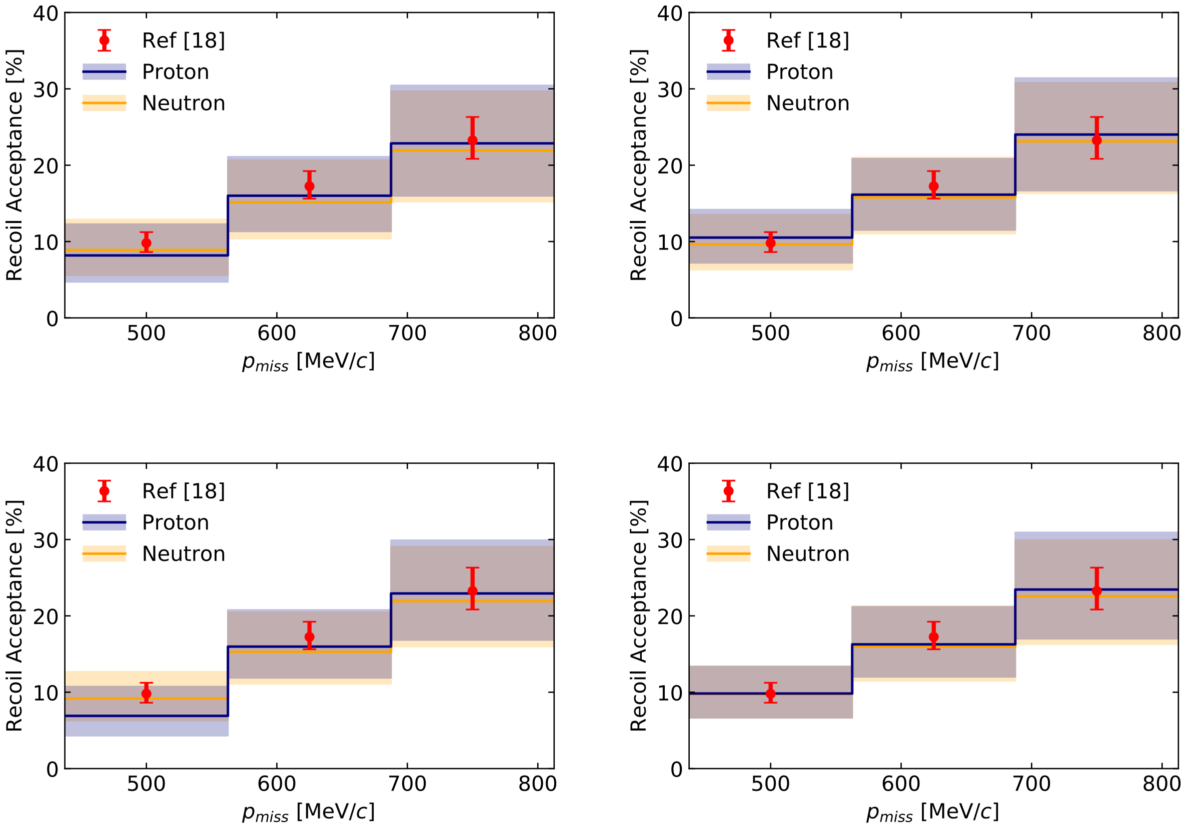


**Supplementary Materials Fig. 6:** Recoil nucleon acceptance correction factors for $^{4}$He(e,e’pN) reaction as calculated in the original publication (data points) and using the light-cone (left) and instant form (right) GCF calculations suing AV18 (top) and N2LO (bottom).

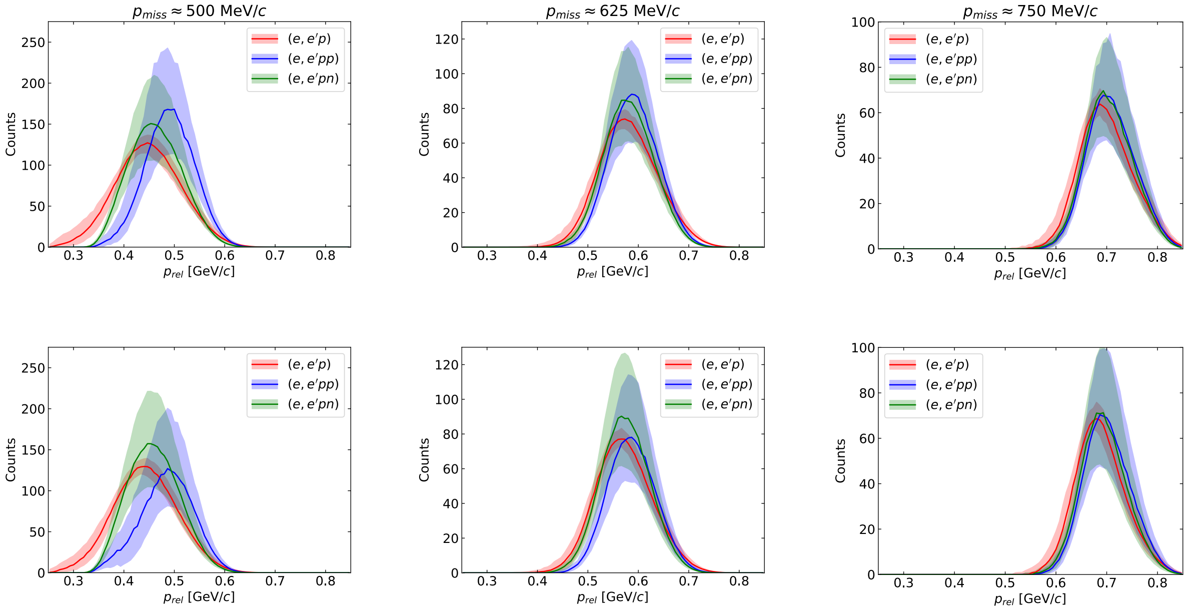


**Supplementary Materials Fig. 7:** GCF calculated pair relative momentum distributions for different kinematical settings. The calculations use the instant form GCF formulation with the AV18 (top) and N2LO (bottom) interactions.

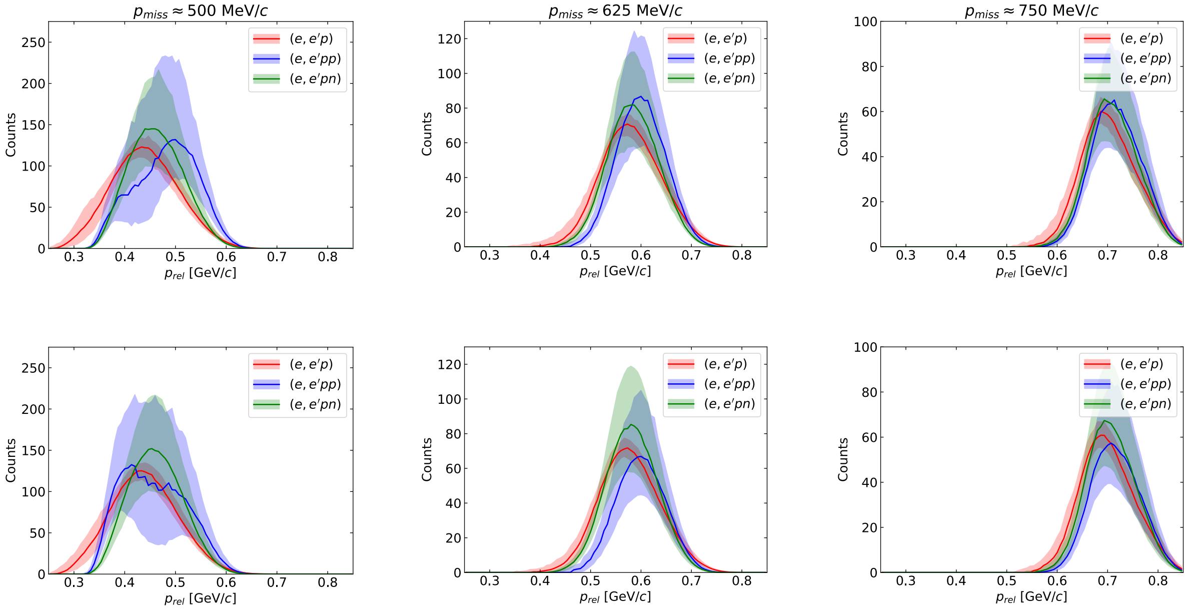


**Supplementary Materials Fig. 8:** Same as Fig. 7 but for light-cone GCF calculations..

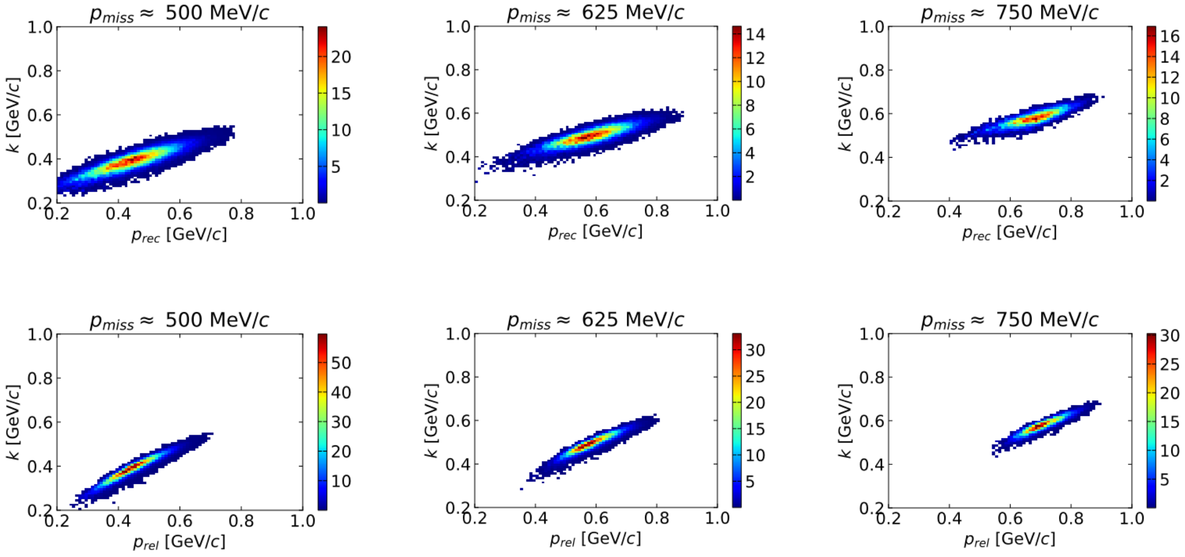


**Supplementary Materials Fig. 9:** GCF calculated correlation between light-cone relative moment k (paper Eq. 10) and recoil nucleon momentum (top) or pair relative momentum (bottom) for the three different measurement kinematics. The calculations use the AV18 NN interaction model.

**Supplementary Materials Table I:** Contributions to theoretical uncertainties resulting from different model parameters. Uncertainty was calculated for event yields and yield ratios, averaged over kinematical settings. Uncertainties below 2% are indistinct from statistical calculation uncertainty. Calculations below were performed using AV18 and instant-form calculations.

| | (e,e'p) Yield | (e,e'pn) Yield | (e,e'pp) Yield | (e,e'pn)/ (e,e'p) | (e,e'pp)/ (e,e'p) | (e,e'pp)/ (e,e'pn) |
|---|---|---|---|---|---|---|
| $\sigma_{CM}$ | <2% | 24.2% | 24.2% | 22.5% | 22.8% | <2% |
| Nuclear Contacts | 6.1% | 6.6% | 9.3% | <2% | 9.8% | 11.7% |
| SCX Probabilities | <2% | 2.3% | 9.9% | <2% | 10.3% | 12.2% |
| Nuclear Transparency | 20% | 28.3% | 28.3% | 20% | 20% | 0% |
| $k_{cut\text{-}off}$ | <2% | <2% | <2% | <2% | <2% | <2% |
| E* | <2% | <2% | 2.1% | <2% | <2% | <2% |

**Supplementary Materials Table II:** Same as Table I but for N2LO and instant-form calculations.

| | (e,e'p) Yield | (e,e'pn) Yield | (e,e'pp) Yield | (e,e'pn)/ (e,e'p) | (e,e'pp)/ (e,e'p) | (e,e'pp)/ (e,e'pn) |
|---|---|---|---|---|---|---|
| $\sigma_{CM}$ | <2% | 20.9% | 21.6% | 21.9% | 23.0% | 2.2% |
| Nuclear Contacts | 8.3% | 9.4% | 11.4% | 2.4% | 11.8% | 13.6% |
| SCX Probabilities | <2% | 2.2% | 13.4% | 2.0% | 13.5% | 15.6% |
| Nuclear Transparency | 20% | 28.3% | 28.3% | 20% | 20% | 0% |
| $k_{cut\text{-}off}$ | <2% | <2% | <2% | <2% | <2% | <2% |
| E* | <2% | <2% | 2.3% | <2% | 2.3% | 2.1% |

**Supplementary Materials Table III:** Same as Table I but for AV18 and light-cone calculations.

| | (e,e'p) Yield | (e,e'pn) Yield | (e,e'pp) Yield | (e,e'pn)/ (e,e'p) | (e,e'pp)/ (e,e'p) | (e,e'pp)/ (e,e'pn) |
|---|---|---|---|---|---|---|
| $\sigma_{CM}$ | 3.0% | 24.4% | 24.9% | 23.8% | 24.5% | 2.4% |
| Nuclear Contacts | 6.6% | 6.9% | 8.4% | <2% | 9.1% | 9.9% |
| SCX Probabilities | <2% | 2.2% | 17.0% | <2% | 17.5% | 19.2% |
| Nuclear Transparency | 20% | 28.3% | 28.3% | 20% | 20% | 0% |
| $k_{cut\text{-}off}$ | <2% | <2% | <2% | <2% | <2% | <2% |
| E* | <2% | <2% | <2% | <2% | 2.8% | 2.3% |

**Supplementary Materials Table IV:** Same as Table I but for N2LO and light-cone calculations.

| | (e,e'p) Yield | (e,e'pn) Yield | (e,e'pp) Yield | (e,e'pn)/ (e,e'p) | (e,e'pp)/ (e,e'p) | (e,e'pp)/ (e,e'pn) |
|---|---|---|---|---|---|---|
| $\sigma_{CM}$ | 2.2% | 21.4% | 22.6% | 22.4% | 24.0% | 2.8% |
| Nuclear Contacts | 9.3% | 9.9% | 10.5% | <2% | 11.1% | 11.9% |
| SCX Probabilities | <2% | 2.1% | 22.0% | <2% | 22.6% | 24.5% |
| Nuclear Transparency | 20% | 28.3% | 28.3% | 20% | 20% | 0% |
| $k_{cut\text{-}off}$ | <2% | <2% | <2% | <2% | 2.1% | 2.2% |
| E* | 2.1% | <2% | 2.1% | <2% | 2.9% | 2.5% |
